# Supplementary material for: Disentangling the Electronic and Lattice Contributions to the Dielectric Response of Photoexcited Bismuth
Source: arXiv:2310.17510 source file (2023-10-26)
Supplement: Supplementary file 1 [file SuppMat.pdf]

# Supplemental Material for "Disentangling the Electronic and Lattice Contributions to the Dielectric Response of Photoexcited Bismuth"

F. Thiemann,[1,*] G. Sciaini,[2] A. Kassen,[1] T.S. Lott,[2] and M. Horn-von Hoegen[1,3]

[1] *Department of Physics, University of Duisburg-Essen, Lotharstrasse 1, 47057 Duisburg, Germany*

[2] *The Ultrafast Electron Imaging Lab, Department of Chemistry, and Waterloo Institute for Nanotechnology, University of Waterloo, Waterloo, Ontario N2L 3G1, Canada*

[3] *Center for Nanointegration (CENIDE), University of Duisburg-Essen, Carl-Benz-Str. 199, 47057 Duisburg, Germany*

(Dated: October 2023)

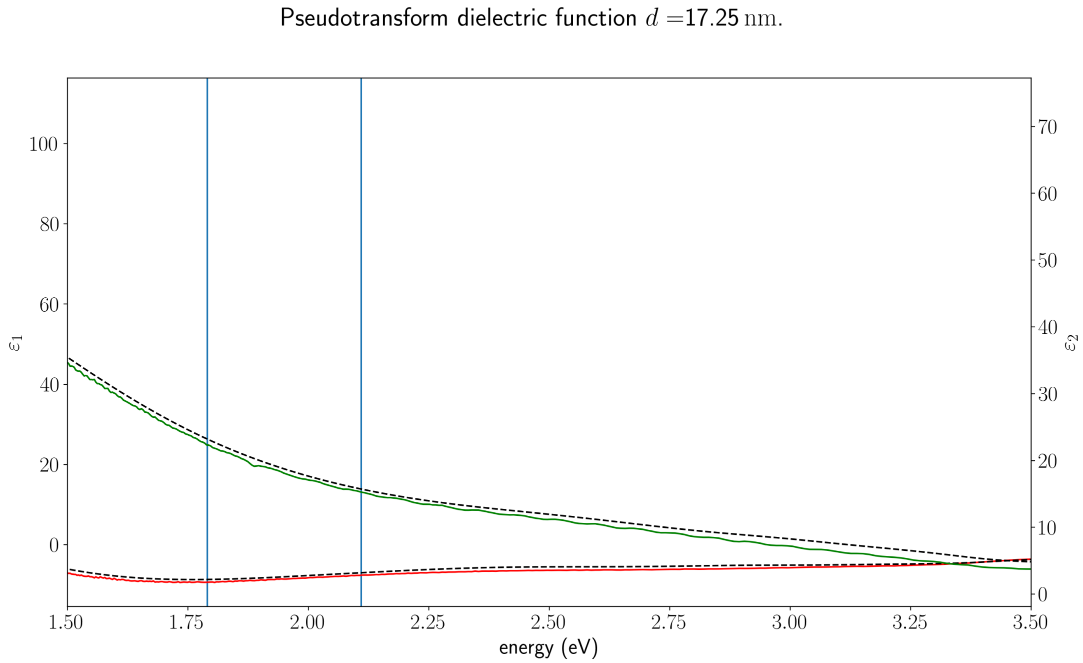


Figure 1: Real ($\varepsilon_1$) and imagninary part ($\varepsilon_2$) of the dielectric function pseudotransformation for the 17 nm sample. The red and green curves mark the data, whereas the dashed line the fits respectively. The blue vertical lines mark the spectral window studied in this work.

## I. ELLIPSOMETRY MEASUREMENTS

To verify if we can perform the analysis comparing the changes in all of the films we conducted ellipsometry measurements on all of the films. The raw data was analysed with the *CompleteEASE* from *J.A. Woollam Co.* [1] yielding the pseudotransformation of the dielectric function of the whole Bi/Si system. This dielectric function was fitted using the transfer matrix model [2], a model for bismuth's dielectric function from literature by Toudert *et al.* [3] and data for the dielectric function of silicon by Herzinger *et al.* [4]. The model for Bi consists of multiple Lorentz oscillators. The film thickness serves as the main fit parameter. The thicknesses we obtain matches with the thicknesses measured during preparation of the films using a quartz balance. The pseudotransformations (red and green curves) are shown in Fig. 1 - 5 with its corresponding fits (dashed lines).

Since the current models from literature describe all of our observations, while reproducing the thicknesses of the films as well, we conclude that we can compare the dielectric function changes introduced by photoexcitation.

* fabian.thiemann@uni-due.de

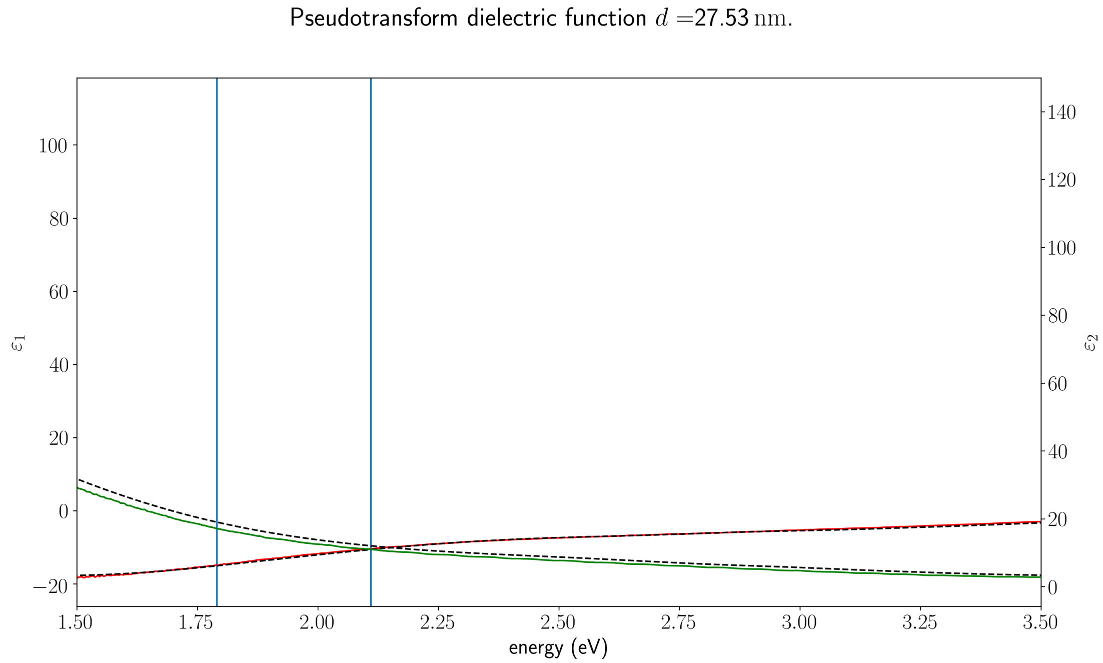


Figure 2: Real ($\varepsilon_1$) and imagninary part ($\varepsilon_2$) of the dielectric function pseudotransformation for the 17 nm sample. The red and green curves mark the data, whereas the dashed line the fits respectively. The blue vertical lines mark the spectral window studied in this work.


[1] Completeease ellipsometry software, j.a. woollam co.

[2] C. C. Katsidis and D. I. Siapkas, Applied Optics **41**, 3978 (2002).

[3] J. Toudert, R. Serna, I. Camps, J. Wojcik, P. Mascher, E. Rebollar, and T. A. Ezquerra, The Journal of Physical Chemistry C **121**, 3511 (2017).

[4] C. M. Herzinger, B. Johs, W. A. McGahan, J. A. Woollam, and W. Paulson, Journal of Applied Physics **83**, 3323 (1998).

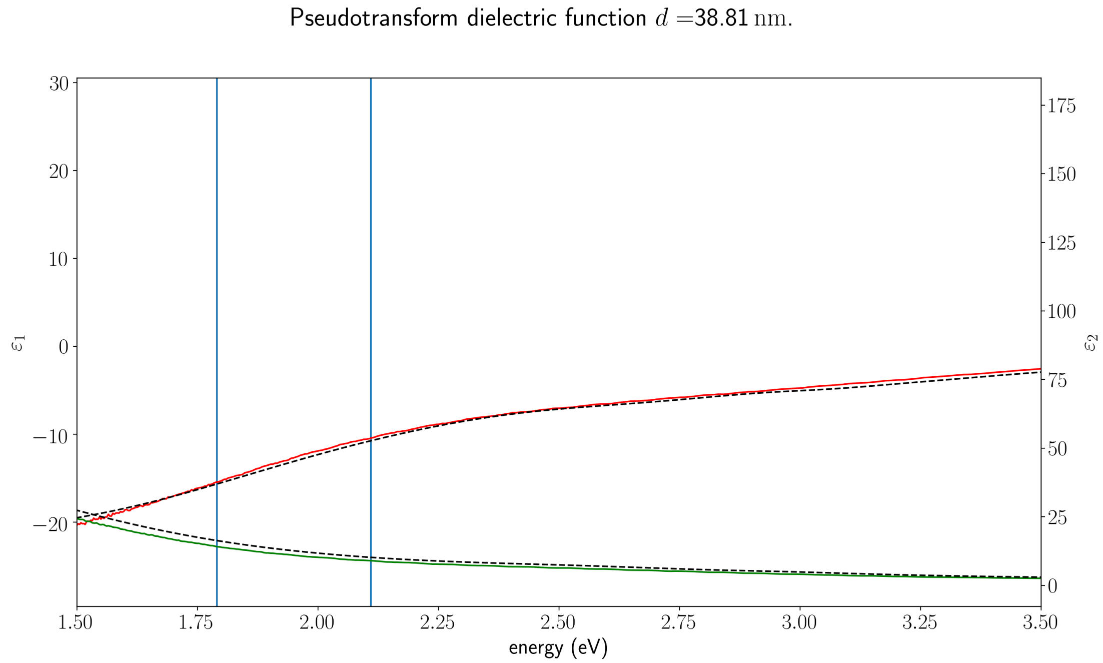


Figure 3: Real ($\varepsilon_1$) and imagninary part ($\varepsilon_2$) of the dielectric function pseudotransformation for the 17 nm sample. The red and green curves mark the data, whereas the dashed line the fits respectively. The blue vertical lines mark the spectral window studied in this work.

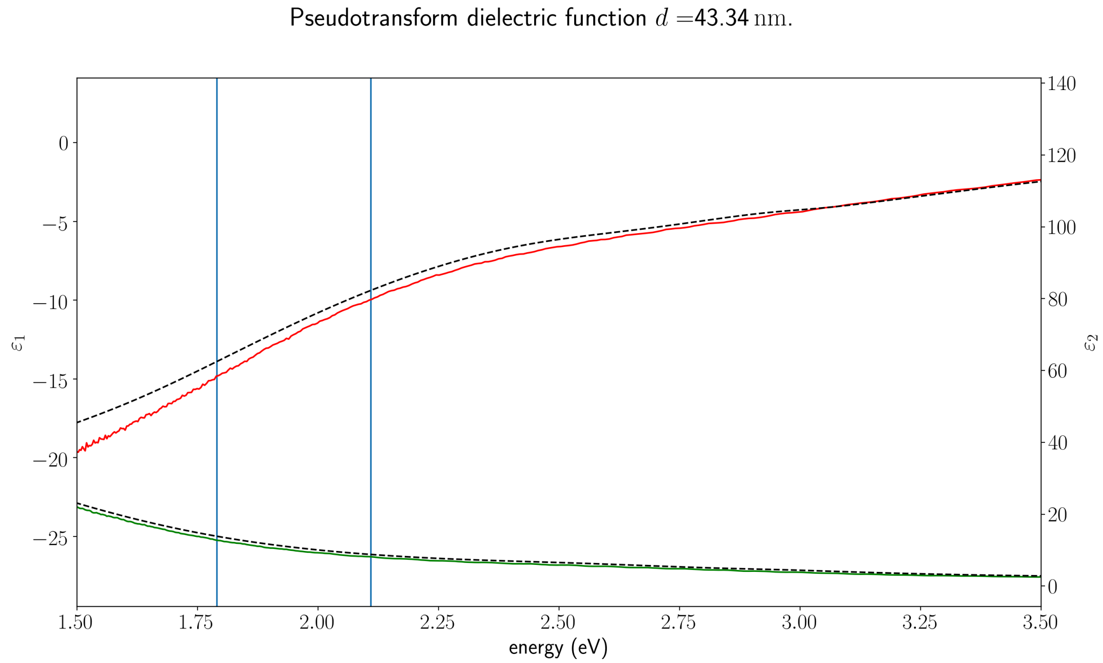


Figure 4: Real ($\varepsilon_1$) and imagninary part ($\varepsilon_2$) of the dielectric function pseudotransformation for the 17 nm sample. The red and green curves mark the data, whereas the dashed line the fits respectively. The blue vertical lines mark the spectral window studied in this work.

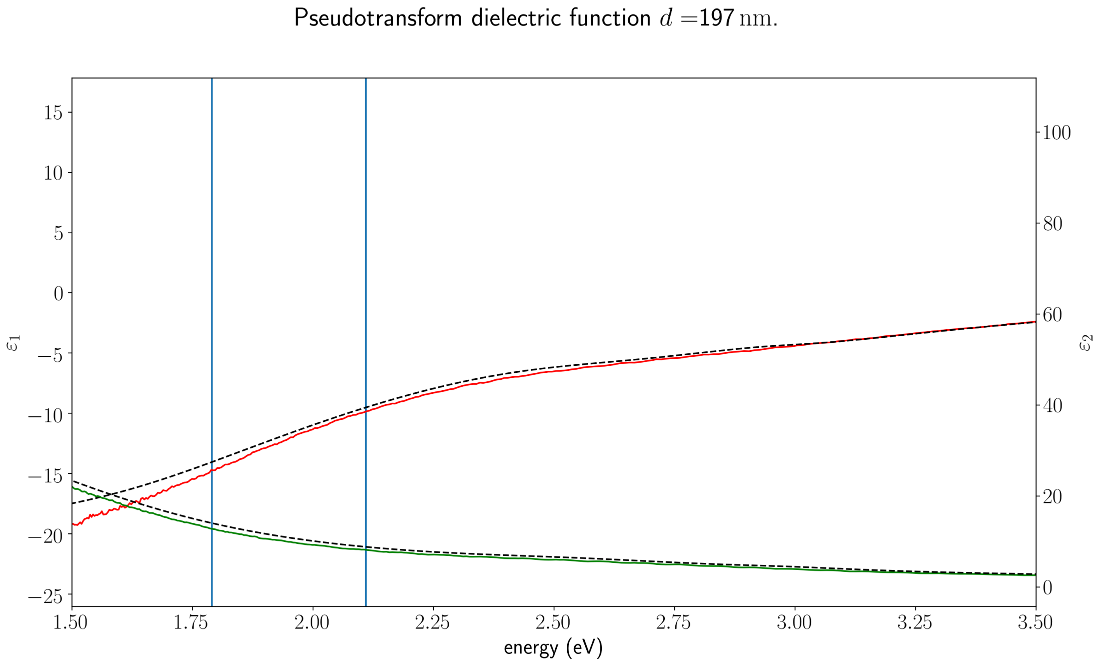


Figure 5: Real ($\varepsilon_1$) and imagninary part ($\varepsilon_2$) of the dielectric function pseudotransformation for the 17 nm sample. The red and green curves mark the data, whereas the dashed line the fits respectively. The blue vertical lines mark the spectral window studied in this work.
